# Supplementary material for: DuetGen: Music Driven Two-Person Dance Generation via Hierarchical Masked Modeling
Source: arXiv:2506.18680 source file (2025-06-23)
Supplement: Supplementary file 1 [file supplementary_document.pdf]

# DuetGen: Music Driven Two-Person Dance Generation via Hierarchical Masked Modeling

## –Appendix–

ANINDITA GHOSH, DFKI, MPI for Informatics, SIC, Germany  
BING ZHOU, Snap Inc., USA  
RISHABH DABRAL, MPI for Informatics, SIC, Germany  
JIAN WANG, Snap Inc., USA  
VLADISLAV GOLYANIK, MPI for Informatics, SIC, Germany  
CHRISTIAN THEOBALT, MPI for Informatics, SIC, Germany  
PHILIPP SLUSALLEK, DFKI, SIC, Germany  
CHUAN GUO, Snap Inc., USA

### ACM Reference Format:

Anindita Ghosh, Bing Zhou, Rishabh Dabral, Jian Wang, Vladislav Golyanik, Christian Theobalt, Philipp Slusallek, and Chuan Guo. 2025. DuetGen: Music Driven Two-Person Dance Generation via Hierarchical Masked Modeling –Appendix–. In *Special Interest Group on Computer Graphics and Interactive Techniques Conference Conference Papers (SIGGRAPH Conference Papers '25)*, August 10–14, 2025, Vancouver, BC, Canada. ACM, New York, NY, USA, 4 pages. <https://doi.org/10.1145/3721238.3730741>

In the appendix, we provide our implementation details, details on the preparation of our baselines, details on the evaluation metrics used, and setup details of our user study.

## A IMPLEMENTATION DETAILS FOR DUETGEN

We provide the implementation details of all our network components, including the hierarchical VQ-VAE, the two-stage masked transformers, and the trajectory refinement module.

*Hierarchical Two-Person Motion VQ-VAE.* We train the hierarchical VQ-VAE for approximately 4K epochs on the DD100 training set using Adam [Kingma and Ba 2014] with a base learning rate (LR) of  $10^{-5}$  and a batch size of 128. Our training data consist of  $N = 400$  frames with  $\eta_{top} = 8$  and  $\eta_{bot} = 4$ . For our codebooks, we use  $K = 1,024$  codes with  $D_{top} = 1,024$  and  $D_{bot} = 512$ . The convolution networks use stride 2 with SiLU [Singh et al. 2023] activations and layer normalization in the ResNet blocks. For the loss terms in

Authors' addresses: Anindita Ghosh, DFKI, MPI for Informatics, SIC, Germany, [anindita.ghosh@dfki.de](mailto:anindita.ghosh@dfki.de); Bing Zhou, Snap Inc., USA, [bzhou@snapchat.com](mailto:bzhou@snapchat.com); Rishabh Dabral, MPI for Informatics, SIC, Germany, [rdabral@mpi-inf.mpg.de](mailto:rdabral@mpi-inf.mpg.de); Jian Wang, Snap Inc., USA, [jwang4@snapchat.com](mailto:jwang4@snapchat.com); Vladislav Golyanik, MPI for Informatics, SIC, Germany, [golyanik@mpi-inf.mpg.de](mailto:golyanik@mpi-inf.mpg.de); Christian Theobalt, MPI for Informatics, SIC, Germany, [theobalt@mpi-inf.mpg.de](mailto:theobalt@mpi-inf.mpg.de); Philipp Slusallek, DFKI, SIC, Germany, [philipp.slusallek@dfki.de](mailto:philipp.slusallek@dfki.de); Chuan Guo, Snap Inc., USA, [cguo2@snapchat.com](mailto:cguo2@snapchat.com).

Permission to make digital or hard copies of all or part of this work for personal or classroom use is granted without fee provided that copies are not made or distributed for profit or commercial advantage and that copies bear this notice and the full citation on the first page. Copyrights for components of this work owned by others than the author(s) must be honored. Abstracting with credit is permitted. To copy otherwise, or republish, to post on servers or to redistribute to lists, requires prior specific permission and/or a fee. Request permissions from [permissions@acm.org](mailto:permissions@acm.org).

*SIGGRAPH Conference Papers '25, August 10–14, 2025, Vancouver, BC, Canada*

© 2025 Copyright held by the owner/author(s). Publication rights licensed to ACM.

ACM ISBN 979-8-4007-1540-2/2025/08

<https://doi.org/10.1145/3721238.3730741>

Table A.1. **Evaluation sweep at inference.** We conduct a systematic analysis of our iterative masked sampling strategies. At 20 iterations, an optimal balance between diversity and fidelity is observed.

| Iterations | FID ↓       | Div →        | PFID ↓      |
|------------|-------------|--------------|-------------|
| 5          | 2.11        | 15.85        | 3.76        |
| 10         | 1.46        | 15.79        | 3.14        |
| 20         | <b>1.31</b> | <b>15.71</b> | <b>2.54</b> |
| 30         | 1.43        | 15.51        | 2.68        |
| 40         | 1.43        | 15.50        | 2.72        |

Equation (8), we experimentally determine the scalar weights as  $\lambda_r = 1.0$ ,  $\lambda_v = 10.0$ ,  $\beta_1, \beta_2 = 1.0$ ,  $\lambda_{com} = 0.1$ ,  $\lambda_{fk} = 2.0$ , and  $\lambda_{rel} = 5.0$ , and apply  $\mathcal{L}_{fk}$  and  $\mathcal{L}_{rel}$  only after 7K training iterations. Training takes approximately 22 hours on an NVIDIA Tesla V100S 32GB GPU.

*Two-Stage Masked Transformer.* We train each stage for approximately 1.6K epochs using Adam with a base LR of  $10^{-5}$  and a batch size of 64. We decay the learning rate using a Step LR scheduler with a step size of 100 epochs and a decay rate of 0.99. We use a 512-dimensional latent embedding and 8 layers in our transformer encoder with 8 attention heads. During inference, we use a CFG scale of 3 with  $L_{top}, L_{bot} = 20$ . Table A.1 shows that 20 iterations strike the optimal balance between diversity and quality, with additional steps ( $> 20$  iterations) yielding diminishing effects. Training takes approximately 12 hours for each transformer on an NVIDIA Tesla V100S 32GB GPU.

*Trajectory Refinement Module.* The refinement network uses 5 convolution layers with stride 2, SiLU activations, and layer normalization in the ResNet blocks, with a latent dimension of 512.

In total, the number of trainable parameters in our full pipeline is  $\sim 172.6$  M. Using our full pipeline, we can generate a dance sequence of 400 frames from a 13.3 seconds music clip in  $\sim 1.43$  seconds.

## B ADDITIONAL DETAILS ON BASELINE PREPARATION

As mentioned in Section 4.1 in the main paper, we use the most relevant motion synthesis methods adaptable to two-person dance

generation: Duolando [Siyao et al. 2024], GCD [Le et al. 2023a], InterGen [Liang et al. 2024], and MoFusion [Dabral et al. 2023]. Here, we detail on how we use each of these methods in our setting.

**Duolando [Siyao et al. 2024].** Duolando is a two-stage framework originally trained on DD100 to generate a follower’s dance motion in harmony with the music and a leader’s dance. In the first stage, four VQ-VAE networks are trained to encode and quantize different parts of the body (upper half, lower half, left hand, right hand) separately for both leader and follower, and another VQ-VAE quantizes the relative translation between the two bodies. In the second stage, a GPT is used to learn the follower’s dance sequence in the quantized code domain based on music and the leader’s codes. At the end, an off-policy reinforcement learning module is employed to fine-tune the network. We keep this framework as it is and use their pre-trained weights to generate our second dancer’s movements from the input music and the first dancer’s movements. Since we do not have an input lead dancer in our case, we train a separate transformer model to generate the lead dancer’s motion from music. For the transformer, we use 4 blocks, each with the latent dimension set to 512 and the attention layer consisting of 4 heads. We encode the music using our condition encoder  $E_M$ . We use a similar motion representation to Duolando, and train the transformer to learn the leader’s motion from the DD100 dataset. We train for 20K iterations on an NVIDIA RTX A4000 GPU and use the Adam optimizer [Kingma and Ba 2014] with a base learning rate of  $10^{-3}$ , a cosine LR scheduler, and a batch size of 64. We use the motion reconstruction loss and velocity loss to train this transformer module. Once this transformer is trained, we insert this module before the original Duolando framework to obtain the follower’s motions.

**GCD [Le et al. 2023a].** GCD utilizes a diffusion-based generative approach to enable the synthesis of a flexible number of dancers from input music. It proposes a Group Contrastive Diffusion (GCD) strategy to enhance the connection between dancers and their group. GCD was originally trained on the AIOZ-GDANCE dataset [Le et al. 2023b] for variable-size group choreography. We re-train this method on the DD100 dataset by setting the number of dancers to 2 and conditioning on the Jukebox [Dhariwal et al. 2020] music features following the original work. We use a 512-dimensional latent embedding for all attention layers with 8 attention heads. We train GCD with 1,000 diffusion steps with cosine noise scheduling, for 500K iterations, on an NVIDIA RTX A4000 GPU. We use the Adam optimizer [Kingma and Ba 2014] with a base learning rate of  $10^{-5}$ , a cosine LR scheduler, and a batch size of 64. During inference, we use the DDIM [Song et al. 2020] sampling strategy with 50 timesteps.

**InterGen [Liang et al. 2024].** InterGen is a diffusion-based approach that generates two-person motions from text prompts. It was originally trained by conditioning on rich textual annotations. It uses cooperative denoisers with novel weight-sharing and a mutual attention mechanism to improve interactions between two persons. To use it as a baseline in our dance generation setting, we replace the conditioning text with conditioning music signals. This is done by replacing the CLIP [Radford et al. 2021] based text encoder module with our proposed music encoder module  $E_M$ . We use

the non-canonical two-person motion representation proposed in the original paper [Liang et al. 2024]. We implement InterGen with 8 transformer blocks with the latent dimension set to 1,024, and each attention layer consisting of 8 heads, as done in the original paper. The number of diffusion timesteps is set to 1,000 during training. We adopt the cosine noise level schedule and classifier-free guidance of 10% during training. Retraining InterGen on the DD100 for 30K iterations takes about 17 hours on a NVIDIA RTX A4000 GPU. We use the Adam optimizer [Kingma and Ba 2014] with a base learning rate of  $10^{-4}$ , a cosine LR scheduler, and a batch size of 64. During inference, we use the DDIM [Song et al. 2020] sampling strategy with 50 timesteps and a guidance scale of 3.5 for the CFG.

**MoFusion [Dabral et al. 2023].** MoFusion uses a lightweight 1D U-Net [Ronneberger et al. 2015] architecture within a denoising diffusion probabilistic model to generate high-quality single-person motion, and the motions can be conditioned on both text or music signals. To use it as a baseline for our two-person dance generation setting, we represent the two-person motion by concatenating the root-relative 3D joint position of each person. The second person is represented as a copy of the first person. We use a latent dimension of 1024 in the audio encoder that takes melspectrogram as input. In the U-Net model, we use cross-modal transformer blocks with 16 attention heads and a cross-attention dimension of 1024. Retraining MoFusion on the DD100 dataset for 10K iterations takes about 6 hours on a NVIDIA RTX A4000 GPU. We use the Adam optimizer [Kingma and Ba 2014] with a base learning rate of  $10^{-4}$  and a batch size of 32.

## C COMPUTATION OF EVALUATION METRICS

We provide the computation details of our evaluation metrics.

- **Mean Per Joint Position Error (MPJPE).** MPJPE measures the mean absolute positional difference of a joint  $j$  between the ground-truth and the generated pose sequences, as

$$MPJPE = \frac{1}{JN} \sum_{n \in N} \sum_{j \in J} \|p_{n,j} - \hat{p}_{n,j}\|_2, \quad (C.1)$$

where  $N$  and  $J$  are the number of frames and number of joints of each person. We report the MPJPE separately for each person.

- **Mean Per Frame Per Joint Velocity Error (MPJVE).** MPJVE measures the mean joint velocity difference for a joint  $j$  between the ground-truth and the generated pose sequences, as

$$MPJVE = \frac{1}{JN} \sum_{n \in N-1} \sum_{j \in J} \|\Delta p_{n,j} - \Delta \hat{p}_{n,j}\|_2, \quad (C.2)$$

where  $N$  and  $J$  are the number of frames and number of joints of each person. We report the MPJVE separately for each person.

- **Relative Distance Error (RDE).** RDE measures the mean absolute difference between the root positions of persons  $\mathcal{A}$  and  $\mathcal{B}$  between the ground-truth and the generated pairs, as

$$RDE = \frac{1}{N} \sum_{n \in N} \|d(p_{\mathcal{A}_n}, p_{\mathcal{B}_n}) - d(\hat{p}_{\mathcal{A}_n}, \hat{p}_{\mathcal{B}_n})\|_2, \quad (C.3)$$

where  $d(\cdot, \cdot)$  is the Euclidean distance between the root joint positions of  $\mathcal{A}$  and  $\mathcal{B}$ .

- **Fréchet Inception Distance (FID)** [Heusel et al. 2017]. It measures the distributional difference between synthesized and real motions for a single person. We pre-train a transformer autoencoder to learn a latent embedding for individual persons’ motion distributions in the DD100 dataset, and use this pre-trained network to get latent embeddings from our generated motions. We then calculate the distributional difference with the ground-truth for each sequence for individual persons. We report the mean value over the test set and average it for the two persons in duet dances.
- **Diversity.** We randomly sample 300 pairs of generated and ground-truth motions, and calculate the average Euclidean distances of these pairs in latent space to measure motion diversity in the generated motion dataset for individual persons. We then report the averaged motion diversity for the two persons.
- **Paired Fréchet Inception Distance score (PFID)** [Ng et al. 2022]. PFID measures the distributional difference between the ground-truth and the generated *paired* motions instead of individual persons’ motions. We pre-train a transformer autoencoder to learn a latent embedding for the concatenated motion representation of the two-person motion distribution in the DD100 dataset, and use this pre-trained network to get latent embeddings from our generated paired motions. We calculate the distributional difference with the ground truth for each paired-motion sequence. We report the mean value over the test set.
- **Physical Foot Contact Score (PFC)** [Tseng et al. 2023]. We measure the realism of foot-ground contact by implementing the metric proposed by [Tseng et al. 2023].
- **Contact Frequency.** We measure the percentage of frames in a sequence where there is contact between the two dancers. We define a frame to have contact if any joint of person  $\mathcal{A}$  has a minimum absolute distance of less than 40 cm with any joint of person  $\mathcal{B}$ . We average it over the entire test set for both the ground-truth and the generated motions.
- **Beat Alignment Score (BAS)** [Tseng et al. 2023]. BAS measures the temporal alignment of dances with the audio beats. We calculate the average temporal distance between each music beat and its closest dance beat, as done in [Siyao et al. 2022]. We average the score for our two-person setting.

## D DETAILS ON USER STUDY SETUP

To evaluate our results, we designed a user study that compares generated dance sequences from our method with generated dance sequences from the three baselines, GCD [Le et al. 2023a], Duolando [Siyao et al. 2024], and InterGen [Liang et al. 2024], on the same input music. Figure D.1 shows the interface we designed for the user study, where participants observe side-by-side comparisons for each set of animations. We asked participants to rate each animation on a 5-point Likert scale based on the following three criteria.

- **Motion Quality.** How natural and plausible do the motions of individual dancers appear? We asked participants to consider artifacts such as implausible poses, broken joints, and foot sliding.
- **Music Alignment.** How well does the generated dance align with the rhythm and mood of the music?
- **Partner Coordination.** How well do the two dancers coordinate with each other? This includes interpretation of the music, synchronization of motions, and alignment of trajectories.

Our participants were between ages 20 and 60, and were from diverse backgrounds in dance expertise. Out of our 30 participants, 3 reported to be experts in dancing, 10 reported to have some intermediate knowledge, and 17 reported to be novices.

## REFERENCES

- Rishabh Dabral, Muhammad Hamza Mughal, Vladislav Golyanik, and Christian Theobalt. 2023. MoFusion: A framework for denoising-diffusion-based motion synthesis. In *Conference on Computer Vision and Pattern Recognition (CVPR)*.
- Prafulla Dhariwal, Heewoo Jun, Christine Payne, Jong Wook Kim, Alec Radford, and Ilya Sutskever. 2020. Jukebox: A generative model for music. *arXiv preprint arXiv:2005.00341* (2020).
- Martin Heusel, Hubert Ramsauer, Thomas Unterthiner, Bernhard Nessler, and Sepp Hochreiter. 2017. Gans trained by a two time-scale update rule converge to a local nash equilibrium. *Advances in neural information processing systems* 30 (2017).
- Diederik P Kingma and Jimmy Ba. 2014. Adam: A method for stochastic optimization. *arXiv preprint arXiv:1412.6980* (2014).
- Nhat Le, Tuong Do, Khoa Do, Hien Nguyen, Erman Tjiputra, Quang D Tran, and Anh Nguyen. 2023a. Controllable group choreography using contrastive diffusion. *ACM Transactions on Graphics (TOG)* 42, 6 (2023), 1–14.
- Nhat Le, Thang Pham, Tuong Do, Erman Tjiputra, Quang D Tran, and Anh Nguyen. 2023b. Music-driven group choreography. In *Proceedings of the IEEE/CVF Conference on Computer Vision and Pattern Recognition*. 8673–8682.
- Han Liang, Wenqian Zhang, Wenxuan Li, Jingyi Yu, and Lan Xu. 2024. InterGen: Diffusion-based multi-human motion generation under complex interactions. *International Journal of Computer Vision* (2024), 1–21.
- Evonne Ng, Hanbyul Joo, Liwen Hu, Hao Li, Trevor Darrell, Angjoo Kanazawa, and Shiry Ginossar. 2022. Learning to listen: Modeling non-deterministic dyadic facial motion. In *Proceedings of the IEEE/CVF Conference on Computer Vision and Pattern Recognition*. 20395–20405.
- Alec Radford, Jong Wook Kim, Chris Hallacy, Aditya Ramesh, Gabriel Goh, Sandhini Agarwal, Girish Sastry, Amanda Askell, Pamela Mishkin, Jack Clark, et al. 2021. Learning transferable visual models from natural language supervision. In *International conference on machine learning*. PMLR, 8748–8763.
- Olaf Ronneberger, Philipp Fischer, and Thomas Brox. 2015. U-net: Convolutional networks for biomedical image segmentation. In *Medical image computing and computer-assisted intervention—MICCAI 2015: 18th international conference, Munich, Germany, October 5–9, 2015, proceedings, part III* 18. Springer, 234–241.
- Bharat Singh, Suchit Patel, Ankit Vijayvargiya, and Rajesh Kumar. 2023. Analyzing the impact of activation functions on the performance of the data-driven gait model. *Results in Engineering* 18 (2023), 101029.
- Li Siyao, Tianpei Gu, Zhitao Yang, Zhengyu Lin, Ziwei Liu, Henghui Ding, Lei Yang, and Chen Change Loy. 2024. Duolando: Follower GPT with Off-Policy Reinforcement Learning for Dance Accompaniment. In *International Conference on Learning Representations (ICLR)*.
- Li Siyao, Weijiang Yu, Tianpei Gu, Chunze Lin, Quan Wang, Chen Qian, Chen Change Loy, and Ziwei Liu. 2022. Bailando: 3d dance generation by actor-critic gpt with choreographic memory. In *Proceedings of the IEEE/CVF Conference on Computer Vision and Pattern Recognition*. 11050–11059.
- Jiaming Song, Chenlin Meng, and Stefano Ermon. 2020. Denoising diffusion implicit models. *arXiv preprint arXiv:2010.02502* (2020).
- Jonathan Tseng, Rodrigo Castellon, and Karen Liu. 2023. EDGE: Editable dance generation from music. In *Conference on Computer Vision and Pattern Recognition (CVPR)*.

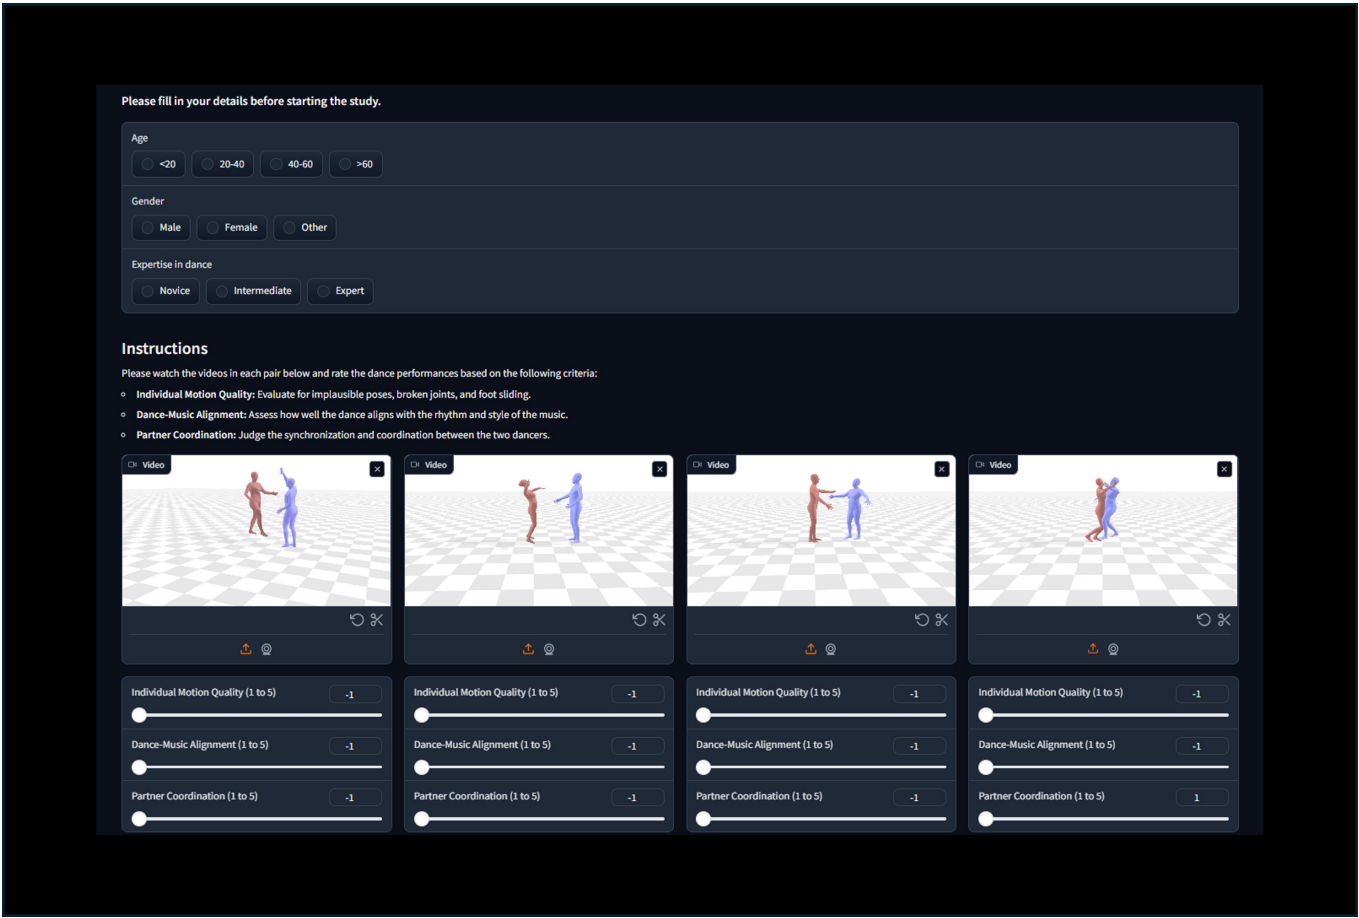

Fig. D.1. **Interface for the User Study.** We designed a user study that shows side-by-side comparisons of the generated dance sequence from our model and our three baselines on the same music.
